# Supplementary material for: Towards Autonomous Navigation in Endovascular Interventions
Source: arXiv:2512.18081 source file (2025-12-23)
Supplement: Supplementary file 1 [file main.tex]

\subsection{CathSim}

This appendix reproduces the full README for \emph{CathSim: An Open-source Simulator for Endovascular Intervention}. For more details, please refer to the project page at \url{https://airvlab.github.io/cathsim/} and the paper at \url{https://arxiv.org/abs/2208.01455}.

\subsubsection{Requirements}

\begin{itemize}
	\item Ubuntu (tested with Ubuntu 22.04 LTS)
	\item Miniconda (tested with Miniconda 23.5)
	\item Python 3.9
\end{itemize}

If \texttt{miniconda} is not installed, run the following script (assuming \texttt{bash} is your shell):

\begin{longlisting}
	\mycaption{Miniconda Installation}{How to install Miniconda.}
	\inputminted[firstline=1]{bash}{postamble/appendices/code/cathsim/code/miniconda_install.sh}
\end{longlisting}

\subsubsection{Installation}

First, create a conda environment and install the package:

\begin{longlisting}
	\mycaption{Create Conda Env}{How to create a conda env.}
	\inputminted{bash}{postamble/appendices/code/cathsim/code/create_env.sh}
\end{longlisting}

\subsubsection{Quickstart}

You can quickly set up a Gym-compatible environment using the \texttt{make\_dm\_env} function along with the \texttt{DMEnvToGymWrapper}. For example:

\begin{longlisting}
	\mycaption{CathSim as Gym Env}{Demonstration of how CathSim can be used as a Gym environment.}
	\inputminted[firstline=1]{python}{postamble/appendices/code/cathsim/code/cathsim_gym.py}
\end{longlisting}

The script creates a \texttt{results} directory in the current working directory and organizes data in a \texttt{<trial\-name>\/<phantom>\/<target>\/<model>} structure. Each model folder contains:

\begin{itemize}
	\item \texttt{eval}: Trajectory data from policy evaluation.
	\item \texttt{models}: Saved PyTorch models.
	\item \texttt{logs}: Tensorboard logs.
\end{itemize}

\subsubsection{Mesh Processing}
To use a custom aorta, perform a V-HACD convex decomposition. A tool called \texttt{stl2mjcf} is available at \url{https://github.com/tudorjnu/stl2mjcf}. To install:

\begin{minted}{bash}
pip install git+git@github.com:tudorjnu/stl2mjcf.git
\end{minted}

After installation, use \texttt{stl2mjcf --help} to see the available commands. Add the resulting XML file to \texttt{cathsim/assets} and the meshes folder to \texttt{cathsim/assets/meshes/}. (You may need to adjust V-HACD parameters for best results.)

\subsubsection{Adding Elements}

\paragraph{Adding a Phantom.} After processing your mesh (see Mesh Processing), add the files to \texttt{src/cathsim/dm/components/phantom\_assets/}. For example, if your phantom is named \texttt{my\_phantom.xml}, you can select it in your code as follows:

\begin{minted}{python}
import cathsim.gym.envs
import gymnasium as gym

task_kwargs = dict(
    phantom="my_phantom",
    target=[0.1, 0.1, 0.1],  # select a target based on the mesh or embed it into the xml
)

env = gym.make("cathsim/CathSim-v0", **task_kwargs)
\end{minted}

For more control, you can manually set up the aorta using the \texttt{mjcf} interface. A more detailed example:

\begin{minted}{python}
from cathsim.gym.envs import CathSim

phantom = MyPhantom()
tip = Tip(n_bodies=4)
guidewire = Guidewire(n_bodies=80)
task = Navigate(
    phantom=phantom,
    guidewire=guidewire,
    tip=tip,
    target=target,
    **kwargs,
)
env = composer.Environment(
    task=task,
    random_state=random_state,
    strip_singleton_obs_buffer_dim=True,
)

env = CathSim(dm_env=env)
\end{minted}

\paragraph{Adding a Guidewire.} A guidewire can be created similarly to the phantom and then integrated into the task. For further details on using \texttt{mjcf}, see \url{https://github.com/google-deepmind/dm_control/tree/main/dm_control/mjcf}.

\subsubsection{Terms of Use}
Please review the project’s \texttt{TERMS.md} before using the software.

\subsubsection{License}
The work is free to copy, distribute, display, perform, or remix for non-commercial purposes only.

% % --- Example Code Listings Section ---
% \section{Code Listings}
%
% \subsection{CathSim Code Sample}
% \begin{quote}
% 	The GitHub repository at \url{https://github.com/airvlab/cathsim} contains the simulator code.
% \end{quote}
%
% \begin{longlisting}
% 	\mycaption{CathSim as Gym Environment}{Demonstration of how CathSim can be used as a Gym environment.}
% 	\label{lst:cathsim-env}\inputminted[firstline=1]{python}{postamble/appendices/cathsim/quickstart.py}
% \end{longlisting}
%
% \begin{longlisting}
% 	\mycaption{CathSim Integration with RL Frameworks}{Demonstration of how CathSim can be integrated with RL frameworks.}
% 	\label{lst:cathsim-rl-training}\inputminted[firstline=1]{python}{postamble/appendices/cathsim/rl_compatibility.py}
% \end{longlisting}
