# Supplementary material for: Towards Autonomous Navigation in Endovascular Interventions
Source: arXiv:2512.18081 source file (2025-12-23)
Supplement: Supplementary file 2 [file appendix.tex]

\appendix
\usemintedstyle{friendly}
\fancyhead[R]{\nouppercase{\itshape Appendix}}

% TODO: Add more visualization
\chapter*{Appendices}
\addcontentsline{toc}{chapter}{Appendices}

% \subimport{appendices/cathsim}{main.tex}
\section{Code Listings}

\section{CathSim}

\subsection{CathSim Design Details}

\textbf{Aortic Models.} In addition to Type-I Aortic Arch model which is mainly used in our experiments, we incorporate three distinct aortic models to enrich our anatomical dataset. These models include a high-fidelity Type-II aortic arch and a Type-I aortic arch with an aneurysm, both sourced from Elastrat, Switzerland. Furthermore, a low tortuosity aorta model, based on a patient-specific CT scan, is included. With these three additional representations, our simulator contains four distinct aorta models. These models aim to enhance the diversity and accuracy of aortic structures available for research and educational endeavors. These aortas are visualized in Fig.~\ref{fig:three aorta}.

\begin{figure}[ht]
	\centering
	\subfloat[Type-I (Aneurysm)]{\includegraphics[width=0.3\textwidth]{assets/aneurysm.png}}
	\hfill
	\subfloat[Type-II]{\includegraphics[width=0.3\textwidth]{assets/type2.png}}
	\hfill
	\subfloat[Low Tortuosity]{\includegraphics[width=0.3\textwidth]{assets/low_tort.png}}
	\caption{Aortic Models.}
	\label{fig:three aorta}
\end{figure}

\subsection{CathSim Speed Evaluation}

\begin{sidebysidefigures}[.5]
	\begin{leftfigure}
		\adjustimage{left}{assets/episode_time.png}
		\captionof{figure}{CathSim training speed.}
		\label{app1fig:fps}
	\end{leftfigure}%
	\begin{rightfigure}
		\vspace{0.35cm}
		\captionof{table}{Comparative training times}\label{app1tab:training-time}
\begin{tabular}{l r r}
	\toprule
	\multirowcell{2}{\thead{Algorithm}} & \multicolumn{2}{c}{\thead{Training Time~(\(\mathbf{\unit{\hour}}\))}}                   \\
	\cmidrule{2-3}
	                                    & \thead{BCA}                                                           & \thead{LCCA}    \\
	\midrule
	Image                               & $3.00 \pm 0.11$                                                       & $2.54 \pm 0.17$ \\
	Image+Mask                          & $4.20 \pm 0.05$                                                       & $4.60 \pm 1.29$ \\
	Internal                            & $2.38 \pm 0.15$                                                       & $2.20 \pm 0.18$ \\
	Internal+Image                      & $3.15 \pm 0.28$                                                       & $3.54 \pm 0.29$ \\
	\textbf{ENN}                        & $4.61 \pm 0.22$                                                       & $4.83 \pm 0.41$ \\
	\bottomrule
\end{tabular}

	\end{rightfigure}

\end{sidebysidefigures}

\paragraph{Training Speed.} As illustrated in Fig.~\ref{app1fig:fps}, we provide a comparison of frames per second (FPS) for the various algorithms we employed during model training. It is evident that utilizing solely the internal state space, comprised of joint positions and velocities, facilitates expedited training processes. In contrast, integrating all modalities into the training process results in its deceleration. The most significant computational demand arises from the dual convolutional neural networks utilized in both the image and mask representations. However, despite this load, the algorithms exhibit respectable computational speed, even during the training phase. Our simulator supports approximately $40$ to $80$ frames per second performance for all implemented algorithms, underscoring the computational speed of our simulation environment. Moreover, we provide the training times in terms of hours for the different modalities in Table~\ref{app1tab:training-time}.

\section{Sim-to-Real Imaging Gap}

We showcase the adaptability of our endovascular simulator using domain adaptation techniques. This is crucial for translating simulated environments into more realistic, X-ray-like images. The implementation of this approach is based on the work of~\autocite{kang2024translating}. Their method, employing multi-scale semantic matching, effectively ensures the preservation of essential structural information in medical images while transitioning from simulated to real-world imaging styles. This technique has demonstrated significant success in producing realistic X-ray images and has set a new benchmark in the field. For an in-depth understanding and visual representation of this adaptation process, we refer readers to the detailed findings and illustrations in the work of~\autocite{kang2024translating}. The adapted images can be visualized in Fig.~\ref{app-fig:sim2real}.

\begin{figure}[h]
	\centering
	\subfloat[]{\includegraphics[width=0.28\linewidth, height=0.28\linewidth]{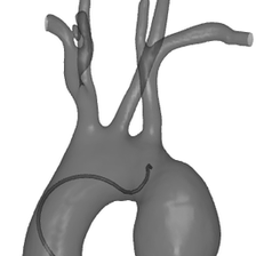}}
	\hspace{1px}
	\subfloat[]{\includegraphics[width=0.28\linewidth, height=0.28\linewidth]{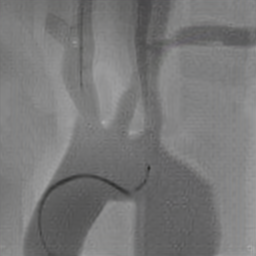}}
	\hspace{1px}
	\subfloat[]{\includegraphics[width=0.28\linewidth, height=0.28\linewidth]{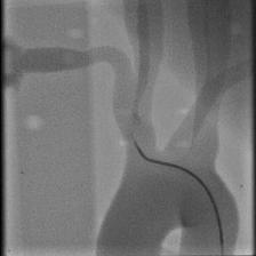}}
	\mycaption{Sim-to-Real Adaptation}{ Demonstration of sim-to-real domain adaptation for creating realistic renderings, featuring \textit{a)} the input image, \textit{b)} the resultant generated image, and \textit{c)} a real X-ray image example. Figure addapted from~\autocite{kang2024translating}}
	\label{app-fig:sim2real}
\end{figure}

\section{Copyright and Reuse Permissions}

Parts of this thesis are based on the author’s previously published work listed below. According to the reuse policies of respective publishers, including Springer Nature and IEEE, authors are permitted to reuse their published material in their thesis or dissertation, provided that proper citation and acknowledgment are included.

\vspace{1em}

\textbf{Springer Nature:} Material from Springer Nature publications is reused in accordance with their author rights policy, which allows reuse of the Version of Record in theses and dissertations. The following acknowledgment applies to all Springer Nature content: \emph{"Reproduced with permission from Springer Nature."}

\vspace{1em}

\textbf{IEEE:} Material from IEEE publications is reused in accordance with IEEE's author rights guidelines, which allow reuse in theses and dissertations under the condition that appropriate copyright notices are included. The IEEE copyright notice ``\emph{\copyright 2024 IEEE. Reprinted, with permission, from [full citation].}'' is provided with any reused material from IEEE publications.

\vspace{1em}

When this thesis is made publicly available, the following notice applies in reference to IEEE copyrighted material:

\begin{quote}
	``In reference to IEEE copyrighted material which is used with permission in this thesis, the IEEE does not endorse any of University of Liverpool products or services. Internal or personal use of this material is permitted. If interested in reprinting/republishing IEEE copyrighted material for advertising or promotional purposes or for creating new collective works for resale or redistribution, please go to \url{http://www.ieee.org/publications_standards/publications/rights/rights_link.html} to learn how to obtain a License from RightsLink. If applicable, University Microfilms and/or ProQuest Library, or the Archives of Canada may supply single copies of the dissertation.''
\end{quote}

\paragraph{Publications Reused in This Thesis:}

\begin{enumerate}
	\item \textbf{Tudor Jianu}, Baoru Huang, Minh Nhat Vu, Mohamed E.M.K. Abdelaziz, Sebastiano Fichera, Chun-Yi Lee, Pierre Berthet-Rayne, Ferdinando Rodriguez y Baena, Anh Nguyen. (2024). \emph{CathSim: An Open-source Simulator for Endovascular Intervention}. \emph{IEEE Transactions on Medical Robotics and Bionics}. IEEE.
	      \emph{\copyright 2024 IEEE. Reprinted, with permission, from the original publication.}

	\item \textbf{Tudor Jianu}, Baoru Huang, Hoan Nguyen, Pierre Berthet-Rayne, Sebastiano Fichera, Anh Nguyen. (2024). \emph{DeepWire: Spherical Coordinate-Based Deep Learning for Accurate Guidewire Shape Reconstruction}. In \emph{Proceedings of the 9th International Conference on Biomedical Signal and Image Processing (ICBIP 2024)}, Suzhou, China.
	      \emph{\copyright 2024 IEEE. Reprinted, with permission, from the original publication.}

	\item \textbf{Tudor Jianu}, Baoru Huang, Pierre Berthet-Rayne, Sebastiano Fichera, Anh Nguyen. (2023). \emph{3D Guidewire Shape Reconstruction from Monoplane Fluoroscopic Images}. \emph{International Conference on Robot Intelligence Technology and Applications}, pp. 84--94. Springer.\\
	      \emph{Reproduced with permission from Springer Nature.}

	\item \textbf{Tudor Jianu}, Baoru Huang, Pierre Berthet-Rayne, Sebastiano Fichera, Anh Nguyen. (2023). \emph{3D Guidewire Shape Reconstruction from Monoplane Fluoroscopic Images}. \emph{11th International Conference on Robot Intelligence Technology and Applications (RiTA)}, 2023.
	      \emph{Reproduced with permission from Springer Nature.}
\end{enumerate}

% \subsection{Additional Related Publications}
%
% \begin{enumerate}
% 	\setcounter{enumi}{2}
% 	\item \textbf{Tudor Jianu}, Baoru Huang, Tuan Vo, Minh Nhat Vu, Jingxuan Kang, Hoan Nguyen, Olatunji Omisore, Pierre Berthet-Rayne, Sebastiano Fichera, Anh Nguyen. (2024). \emph{Autonomous Catheterization with Open-source Simulator and Expert Trajectory}. - [Manuscript/Preprint status depending on final publication].
%
% 	\item Jingxuan Kang, \textbf{Tudor Jianu}, Baoru Huang, Binod Bhattarai, Ngan Le, Frans Coenen, Anh Nguyen. (2023). \emph{Translating Simulation Images to X-ray Images via Multi-Scale Semantic Matching}. arXiv. [Open Access].
% \end{enumerate}

All content reused from published sources is cited appropriately throughout the thesis. Any figures, tables, or excerpts are accompanied by the necessary copyright acknowledgments in their captions or associated text.
