# Supplementary material for: Towards Autonomous Navigation in Endovascular Interventions
Source: arXiv:2512.18081 source file (2025-12-23)
Supplement: Supplementary file 4 [file code_listing.tex]

\begin{longlisting}
	\mycaption{Example Source Code - Add Two Integers}{Python code to perform addition of two integers.}
	\label{lst:add_two_integers} \inputminted[firstline=1]{python}{quickstart.py}
\end{longlisting}

\clearpage
