# Supplementary material for: Towards Autonomous Navigation in Endovascular Interventions
Source: arXiv:2512.18081 source file (2025-12-23)
Supplement: Supplementary file 8 [file network_choice.tex]

\section{Network Choice}\label{app:network-choice}

In our experimental trials, we implemented a transformer-based architecture, drawing inspiration from the visual transformer by~\autocite{dosovitskiy2020image}. This architecture was specifically tailored with an image size of \(80\), a patch size of \(10\), and a single-channel configuration, alongside a depth of \(3\) and \(4\) heads within the attention layers. Despite these specifications, the transformer model did not achieve the expected performance level in our specialized domain of endovascular navigation. It notably struggled to complete the designated tasks within the desired timeframe. This underperformance, coupled with signs of convergence, is illustrated in Fig~\ref{app-fig:vit}, highlighting the challenges encountered in applying this model to our specific context.

\begin{figure}[h]
	\centering
	\includegraphics{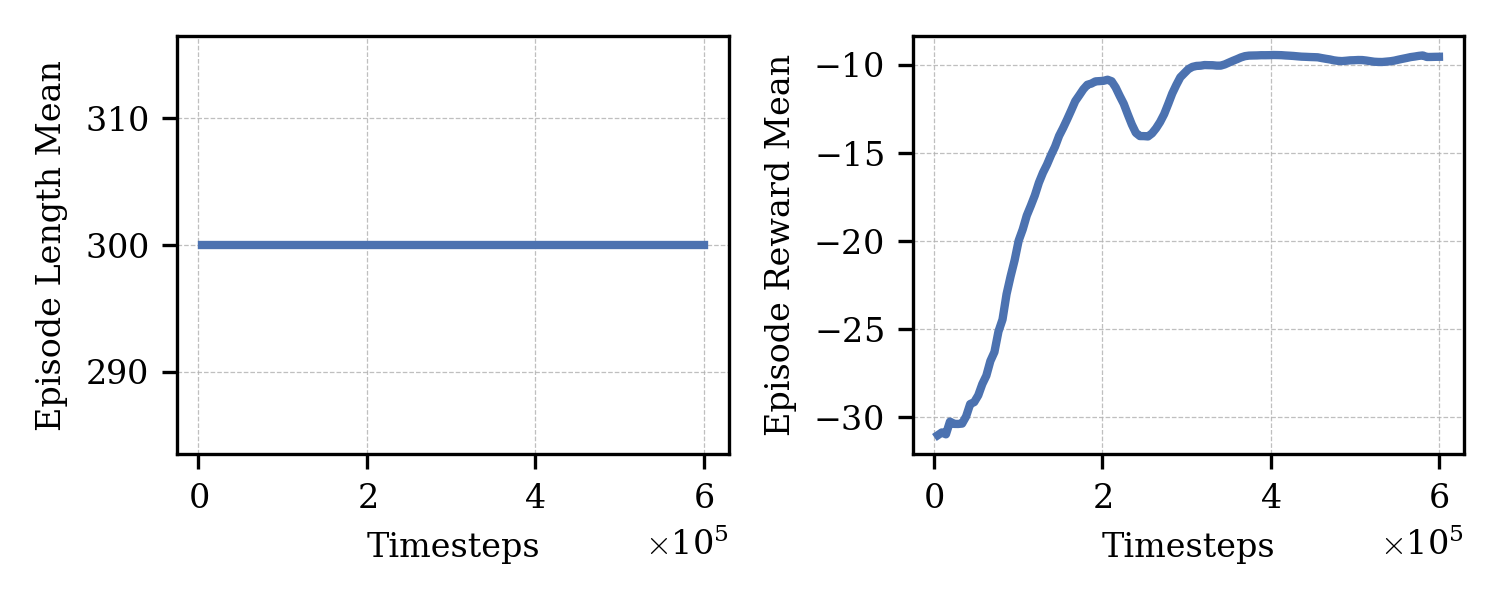}
	\caption{\textbf{ViT-Based ENN Trials:} Initial results indicate that using ViT as a feature extractor does not improve outcomes and fails to meet the target within the time limit, despite showing convergence.}
	\label{app-fig:vit}
\end{figure}
