# Supplementary material for: Towards Autonomous Navigation in Endovascular Interventions
Source: arXiv:2512.18081 source file (2025-12-23)
Supplement: Supplementary file 9 [file sim2real.tex]

\section{Sim-to-Real Imaging Gap}

We showcase the adaptability of our endovascular simulator using domain adaptation techniques. This is crucial for translating simulated environments into more realistic, X-ray-like images. The implementation of this approach is based on the work of~\autocite{kang2024translating}. Their method, employing multi-scale semantic matching, effectively ensures the preservation of essential structural information in medical images while transitioning from simulated to real-world imaging styles. This technique has demonstrated significant success in producing realistic X-ray images and has set a new benchmark in the field. For an in-depth understanding and visual representation of this adaptation process, we refer readers to the detailed findings and illustrations in the work of~\autocite{kang2024translating}. The adapted images can be visualized in Fig.~\ref{app-fig:sim2real}.

\begin{figure}[h]
	\centering
	\subfloat[]{\includegraphics[width=0.28\linewidth, height=0.28\linewidth]{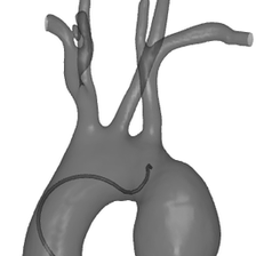}}
	\hspace{1px}
	\subfloat[]{\includegraphics[width=0.28\linewidth, height=0.28\linewidth]{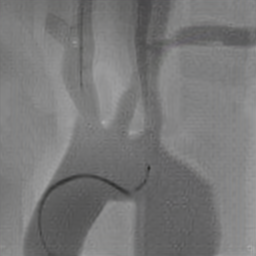}}
	\hspace{1px}
	\subfloat[]{\includegraphics[width=0.28\linewidth, height=0.28\linewidth]{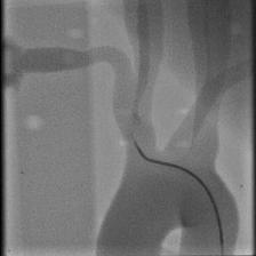}}
	\mycaption{Sim-to-Real Adaptation}{ Demonstration of sim-to-real domain adaptation for creating realistic renderings, featuring \textit{a)} the input image, \textit{b)} the resultant generated image, and \textit{c)} a real X-ray image example. Figure addapted from~\autocite{kang2024translating}}
	\label{app-fig:sim2real}
\end{figure}
