# Supplementary material for: Towards Autonomous Navigation in Endovascular Interventions
Source: arXiv:2512.18081 source file (2025-12-23)
Supplement: Supplementary file 11 [file training_times_coparison.tex]

\captionof{table}{Comparative training times}\label{app1tab:training-time}
\begin{tabular}{l r r}
	\toprule
	\multirowcell{2}{\thead{Algorithm}} & \multicolumn{2}{c}{\thead{Training Time~(\(\mathbf{\unit{\hour}}\))}}                   \\
	\cmidrule{2-3}
	                                    & \thead{BCA}                                                           & \thead{LCCA}    \\
	\midrule
	Image                               & $3.00 \pm 0.11$                                                       & $2.54 \pm 0.17$ \\
	Image+Mask                          & $4.20 \pm 0.05$                                                       & $4.60 \pm 1.29$ \\
	Internal                            & $2.38 \pm 0.15$                                                       & $2.20 \pm 0.18$ \\
	Internal+Image                      & $3.15 \pm 0.28$                                                       & $3.54 \pm 0.29$ \\
	\textbf{ENN}                        & $4.61 \pm 0.22$                                                       & $4.83 \pm 0.41$ \\
	\bottomrule
\end{tabular}
